# Supplementary material for: Preprocessing to Reduce the Search Space for Odd Cycle Transversal
Source: arXiv:2409.00245 source file (2024-10-07)
Supplement: Supplementary file 1 [file a_appendix.tex]

% \section{Proofs}
% \label{sec:appendix1}
